# Supplementary material for: L-C2ST: Local Diagnostics for Posterior Approximations in Simulation-Based Inference
Source: arXiv:2306.03580 source file (2023-10-09)

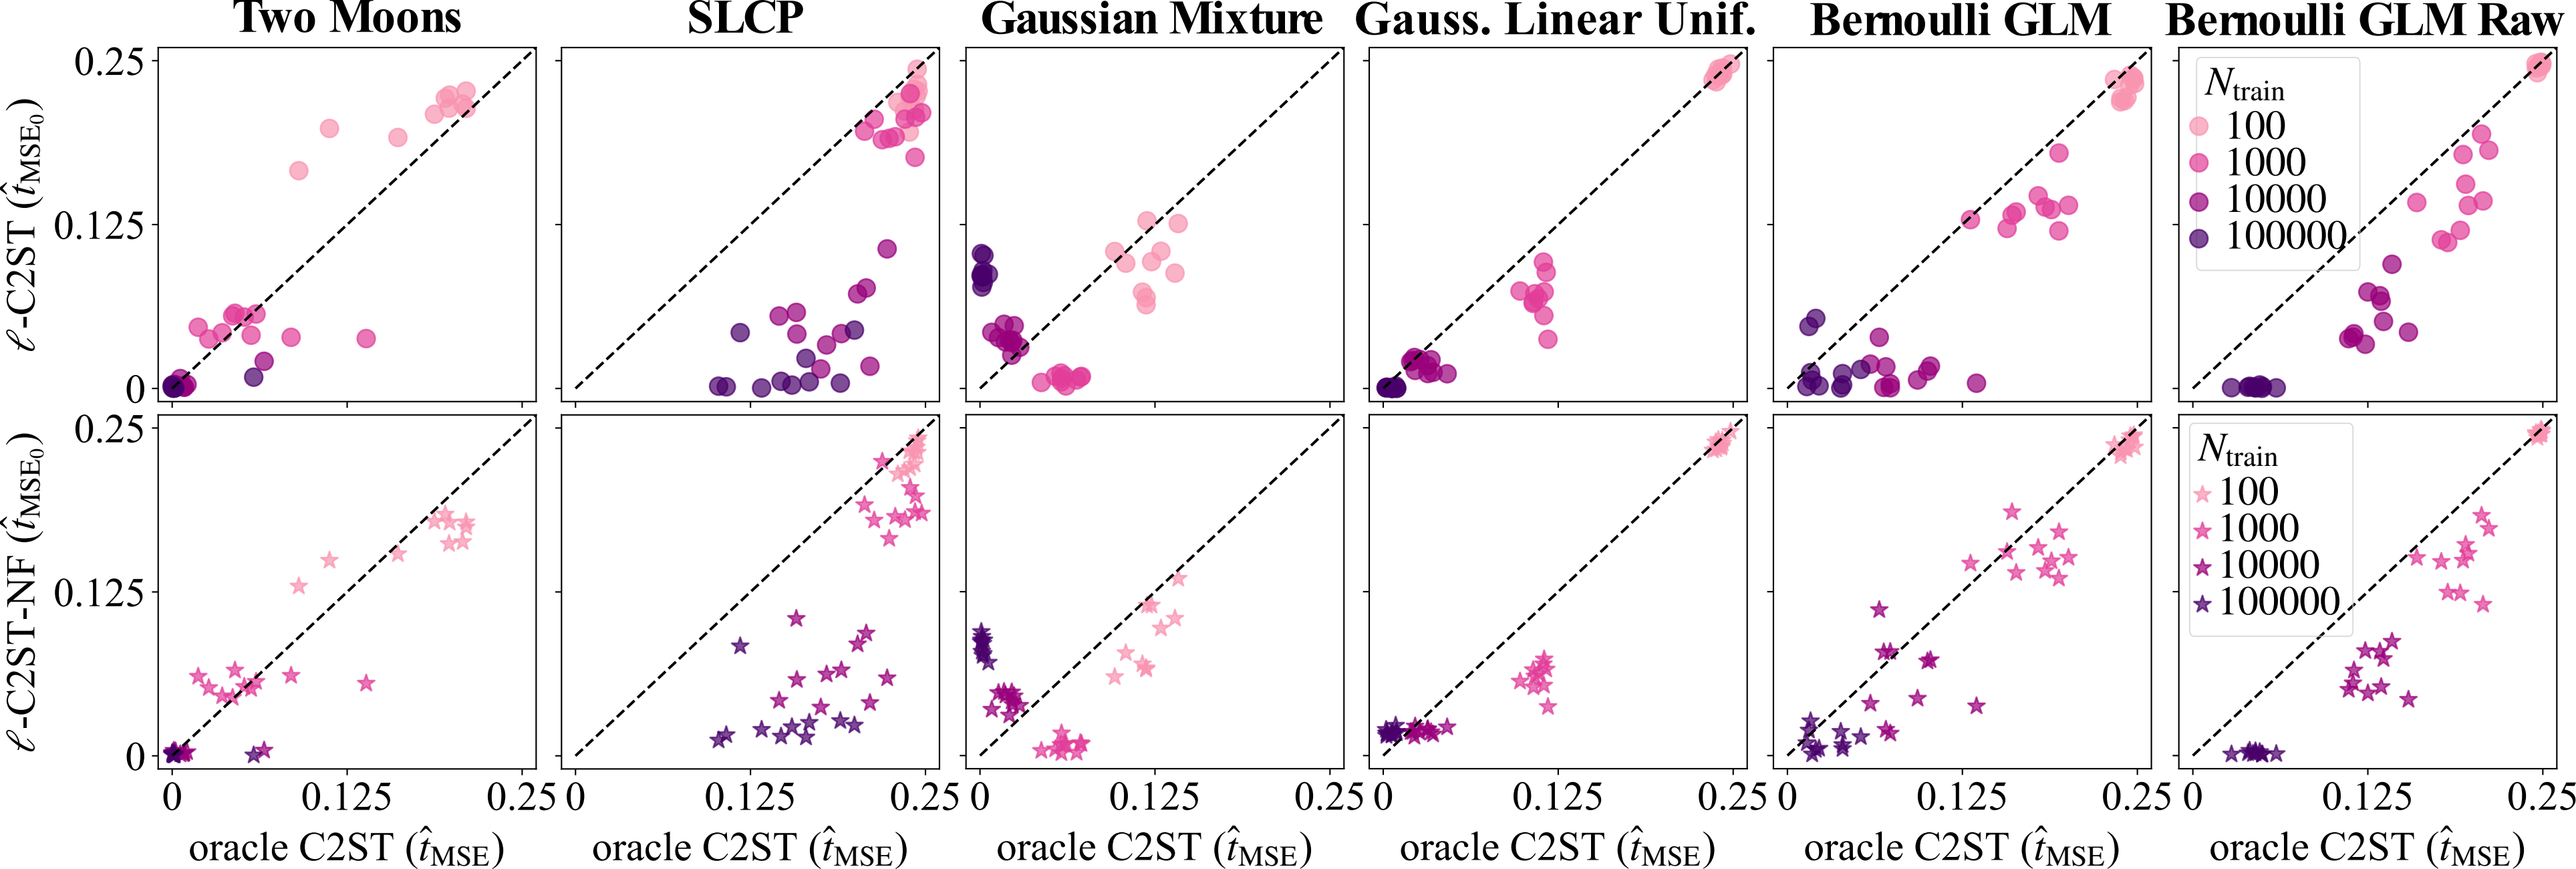

Supplement: Supplementary file 1 [file scatter_final.pdf]
